# Supplementary material for: Characterizing First Arrival Position Channels: Noise Distribution and Capacity Analysis
Source: arXiv:2306.08353 source file (2024-02-17)
Supplement: Supplementary file 1 [file Appendix4.tex]

The theorem can be stated as follows: 
let $p$ be the density of Gaussian distribution $\mathcal{N}(\bs{0},\Sigma)$, i.e., the Gaussian density with zero mean and covariance matrix $\Sigma=[\Sigma_{ij}]$.
Let $q$ be any density satisfying $\int q(\mathbf{x}) x_i x_j \mathrm{d}\mathbf{x}=\Sigma_{i j}$ for all $i,j$. 
Then the differential entropies have the relation: $h(q) \leq h(p)$.
\begin{proof}
Let $A$ be the support of $q(\cdot)$ and $B$ be the support of $p(\cdot)$. Note that $p$ is Gaussian distributed, so that it has full support. So clearly we have $q\ll p$, and the Kullback-Liebler divergence $\mathbb{D}(q \| p)$ is well-defined \cite{yeung2008information,tomamichel2015quantum}.
We can thus deduce that
% $$
\begin{align}
\begin{split}
0 
%& 
\leq 
\mathbb{D}(q \| p)
&
=
\int_A q(\mathbf{x}) \log \frac{q(\mathbf{x})}{p(\mathbf{x})} ~\mathrm{d} \mathbf{x}\\
&=
-h(q)-\int_A q(\mathbf{x}) \log p(\mathbf{x}) ~\mathrm{d} \mathbf{x} 
\\
& 
\overset{(a)}{=}-h(q)-\int_B p(\mathbf{x}) \log p(\mathbf{x}) ~\mathrm{d} \mathbf{x} 
=-h(q)+h(p)    
\end{split}
\end{align}
% $$
where (a) follows since $\log p(\mathbf{x})$ is a quadratic form without linear terms (since $p$ is zero-mean), and by the assumptions, $q$ and $p$ share the same second moments $\Sigma_{ij}$.
\end{proof}
